# Supplementary material for: Collective suppression of optical hyperfine pumping in dense clouds of atoms in microtraps
Source: arXiv:1804.09759 source file (2019-12-05)
Supplement: Supplementary file 1 [file supp_mat-pra.pdf]

# Supplemental material: Collective suppression of optical hyperfine pumping in dense clouds of atoms in microtraps

Shimon Machluf,[1] Julian B. Naber,[1] Maarten L. Soudijn,[1] Janne Ruostekoski,[2] and Robert J. C. Spreeuw[1]

[1] *Van der Waals-Zeeman Institute, Institute of Physics, University of Amsterdam, Science Park 904, 1098XH Amsterdam, The Netherlands*

[2] *Department of Physics, Lancaster University, Lancaster, LA1 4YB, United Kingdom*

In this Supplemental material we provide a more detailed description of the numerical simulation methods that are used to demonstrate the density-dependent suppression of optical pumping. We also explain the image analysis we perform, and how we convert the optical density image to number of atoms.

## SIMULATION DETAILS

In the experiment the atoms are confined in an array of microtraps and occupy the $(5S_{1/2})$ $|F, m_F\rangle = |2,2\rangle$ electronic ground state. An incident laser excites the atoms to the $(5P_{3/2})$ $|F', m_{F'}\rangle = |2,1\rangle$ state from which the atoms decay to either the $F=2$ manifold, with $m_F = 0,1,2$ (of which $m_F=0$ is untrapped), or to untrapped states in the $F=1$ manifold, with $m_F = 0,1$. Reabsorption of light can take the atom to additional levels in the $F=1,2$ and $F'=2$ manifolds. The optical pumping rate is measured by detecting the remaining trapped atoms in the $F=2$ states.

Standard coupled-dipole model simulations [1] are formulated for a single electronic ground level and for the limit of low light intensity where the atoms respond to light as linear harmonic oscillators. The system we are studying involves more than one electronic ground level that participate in optical transitions and the optical pumping necessitates simulation approaches that go beyond the low light intensity limit, incorporating also the excited state dynamics. In order to do this we apply a recently proposed formalism [2] of coupled-dipole model equations that specifically account for the internal level dynamics. This leads to the stochastic electrodynamics of radiatively coupled equations of motion for each atom. We integrate the dynamics within a semiclassical approximation, describing each atom by its own local density matrix $\rho_{ab}^{(j)}$. All the elements for all different atoms $\rho_{ab}^{(j)}$ are radiatively coupled, but quantum entanglement between the atoms is neglected.

The procedure for solving for the optical response of the stochastic electrodynamics of light and atoms amounts to a Monte Carlo integration. In each stochastic realization the discrete atomic positions $\{\mathbf{X}_1, \ldots, \mathbf{X}_N\}$ are randomly sampled from the appropriate spatial distribution. For each such a realization, we solve the coupled electrodynamics for light and atoms at fixed positions. The optical response of the ensemble is then given by averaging quantities of interest over many realizations. The ensemble-averaging establishes spatial correlations between the atoms due to resonant dipole-dipole interactions. The methodology is detailed in Ref. [2].

We introduce a notation where $\hat\rho_{ab}(\mathbf{r})$ denotes a single particle density matrix with $a,b = e,g$ referring to the electronically excited $e$ and ground $g$ levels, where $e$ and $g$ also run over the different Zeeman sublevels, and $\hat\rho_{ab}(\mathbf{r})$ corresponds to the annihilation of an atom in the level $b$ and the creation of an atom in the level $a$. We then write $\hat\rho_{ab}(\mathbf{r})$ for $N$ atoms at fixed positions $\{\mathbf{X}_1, \ldots, \mathbf{X}_N\}$ (corresponding to one particular stochastic realization) as the sum over the atoms $j$,

$$\langle \hat\rho_{ab}(\mathbf{r})\rangle_{\{\mathbf{X}_1,\ldots,\mathbf{X}_N\}} = \sum_j \rho_{ab}^{(j)} \delta(\mathbf{r}-\mathbf{X}_j)\,. \tag{1}$$

Then, e.g., the dipole amplitude for the transition $|g\rangle \leftrightarrow |e\rangle$ is given by

$$\mathbf{d}_{ge}^{(j)} \rho_{ge}^{(j)}(t) = \mathcal{D} \sum_{\sigma=-1}^{1} \mathcal{C}_{g,e}^{(\sigma)} \hat{\mathbf{e}}_\sigma \rho_{ge}^{(j)}(t)\,, \tag{2}$$

and the corresponding positive frequency component of the atomic polarization density

$$\langle \hat{\mathbf{P}}^+\rangle_{\{\mathbf{X}_1,\ldots,\mathbf{X}_N\}} = \sum_j \sum_{ge} \mathbf{d}_{ge}^{(j)} \rho_{ge}^{(j)}(t) \delta(\mathbf{r}-\mathbf{X}_j), \tag{3}$$

where $\mathcal{C}_{g,e}^{(\sigma)} \equiv \langle 1F_g; F_e e | F_g g; 1\sigma\rangle$ are Clebsch-Gordan coefficients for the corresponding dipole transition ($F_f$ is the total atomic angular momentum of hyperfine level $f$), $\mathcal{D}$ is the reduced dipole matrix element, and $\sigma = -1, 0, 1$ is an index indicating the unit circular polarization vectors.

Here and elsewhere in this paper we have assumed that the atoms are illuminated by an incident laser with the dominant frequency $\Omega$, and that all the relevant quantities are expressed as slowly varying amplitudes by explicitly factoring out the laser frequency oscillations by writing $\hat{\mathbf{P}}^+ \to e^{-i\Omega t}\hat{\mathbf{P}}^+$, and similarly for electric displacement $\mathbf{D}^+ \to e^{-i\Omega t}\mathbf{D}^+$ and electric field $\mathbf{E}^+ \to e^{-i\Omega t}\mathbf{E}^+$.

The electric field amplitude may be expressed as the sum of the incident and the scattered fields

$$\epsilon_0 \mathbf{E}^+(\mathbf{r}) = \mathbf{D}_F^+(\mathbf{r}) + \int d^3r'\, \mathsf{G}(\mathbf{r}-\mathbf{r}')\, \mathbf{P}^+(\mathbf{r}')\,, \tag{4}$$

where the monochromatic dipole radiation kernel [3] $\mathsf{G}(\mathbf{r})$ provides the radiated field at $\mathbf{r}$ from a dipole with the amplitude $\hat{\mathbf{d}}$ residing at the origin ($k=\Omega/c$):

$$\mathsf{G}(\mathbf{r})\,\hat{\mathbf{d}} = \frac{k^3}{4\pi}\Big\{(\hat{\mathbf{n}}\times\hat{\mathbf{d}})\times\hat{\mathbf{n}}\frac{e^{ikr}}{kr} + [3\hat{\mathbf{n}}(\hat{\mathbf{n}}\cdot\hat{\mathbf{d}})-\hat{\mathbf{d}}]\big[\frac{1}{(kr)^3}-\frac{i}{(kr)^2}\big]e^{ikr}\Big\} - \frac{\hat{\mathbf{d}}\,\delta(\mathbf{r})}{3}, \quad (5)$$

where $\hat{\mathbf{n}}=\mathbf{r}/r$.

The light mediates strong interactions between the atoms. Each atom is driven by the incident field and the field scattered by all the other atoms in the ensemble. This yields the coupled equations of motion for $\rho^{(j)}_{ab}$ for each atom $j$ and internal levels $a,b$.

We introduce an abbreviated notation for the radiative coupling coefficients between the atoms at the locations $\mathbf{X}_j$ and $\mathbf{X}_l$ as $\mathcal{G}^{(jl)}_{\sigma\varsigma}$ that mediate the interactions between dipoles of orientations $\hat{\mathbf{e}}_\sigma$ and $\hat{\mathbf{e}}_\varsigma$,

$$\mathcal{G}^{(jl)}_{\sigma\varsigma} = \hat{\mathbf{e}}^*_\sigma\cdot\mathsf{G}(\mathbf{X}_j-\mathbf{X}_l)\hat{\mathbf{e}}_\varsigma. \quad (6)$$

We can then derive the equations of motion for the atomic level density matrix elements for each atom $j$ in the ensemble to correspond to the experimental system with one electronically excited level $e$, where the indices $g$ run over all the electronic ground states in the system

$$\frac{d}{dt}\rho^{(j)}_{ge} = (i\Delta_{ge}-\Gamma)\rho^{(j)}_{ge} + i\frac{\xi}{\mathcal{D}}\rho^{(j)}_{gg'}\mathcal{C}^{(\sigma)}_{g',e}\hat{\mathbf{e}}^*_\sigma\cdot\mathbf{D}^+_F(\mathbf{X}_j) - i\frac{\xi}{\mathcal{D}}\rho^{(j)}_{ee}\mathcal{C}^{(\sigma)}_{g,e}\hat{\mathbf{e}}^*_\sigma\cdot\mathbf{D}^+_F(\mathbf{X}_j) + i\xi\sum_{l\neq j}\mathcal{C}^{(\sigma)}_{g',e}\mathcal{G}^{(jl)}_{\sigma\varsigma}\mathcal{C}^{(\varsigma)}_{g'',e}\rho^{(l)}_{g''e}\rho^{(j)}_{gg'} - i\xi\sum_{l\neq j}\mathcal{C}^{(\sigma)}_{g,e}\mathcal{G}^{(jl)}_{\sigma\varsigma}\mathcal{C}^{(\varsigma)}_{g'',e}\rho^{(l)}_{g''e}\rho^{(j)}_{ee}, \quad (7a)$$

$$\frac{d}{dt}\rho^{(j)}_{gg'} = i\Delta_{gg'}\rho^{(j)}_{gg'} + 2\Gamma\mathcal{C}^{(\sigma)}_{g',e}\mathcal{C}^{(\sigma)}_{g,e}\rho^{(j)}_{ee} - i\frac{\xi}{\mathcal{D}}\rho^{(j)}_{eg'}\mathcal{C}^{(\sigma)}_{g,e}\hat{\mathbf{e}}^*_\sigma\cdot\mathbf{D}^+_F(\mathbf{X}_j) + i\frac{\xi}{\mathcal{D}}\rho^{(j)}_{ge}\mathcal{C}^{(\sigma)}_{g',e}\hat{\mathbf{e}}_\sigma\cdot\mathbf{D}^-_F(\mathbf{X}_j) - i\xi\sum_{l\neq j}\mathcal{C}^{(\sigma)}_{g,e}\mathcal{G}^{(jl)}_{\sigma\varsigma}\mathcal{C}^{(\varsigma)}_{g'',e}\rho^{(l)}_{g''e}\rho^{(j)}_{eg'} + i\xi\sum_{l\neq j}\mathcal{C}^{(\sigma)}_{g',e}[\mathcal{G}^{(jl)}_{\sigma\varsigma}]^*\mathcal{C}^{(\varsigma)}_{g'',e}\rho^{(l)}_{eg''}\rho^{(j)}_{ge}, \quad (7b)$$

$$\frac{d}{dt}\rho^{(j)}_{ee} = -2\Gamma\rho^{(j)}_{ee} - 2\mathrm{Im}\big[\frac{\xi}{\mathcal{D}}\rho^{(j)}_{eg}\mathcal{C}^{(\sigma)}_{g,e}\hat{\mathbf{e}}^*_\sigma\cdot\mathbf{D}^+_F(\mathbf{X}_j)\big] - 2\mathrm{Im}\big[\xi\sum_{l\neq j}\mathcal{C}^{(\sigma)}_{g,e}\mathcal{G}^{(jl)}_{\sigma\varsigma}\mathcal{C}^{(\varsigma)}_{g',e}\rho^{(l)}_{g'e}\rho^{(j)}_{eg}\big]. \quad (7c)$$

Here the repeated indices $\sigma,\varsigma$ and the ground state symbols that do not appear on the left-hand-side are implicitly summed over, $\xi=\mathcal{D}^2/(\hbar\epsilon_0)$, $\Gamma$ is the half linewidth at half maximum (HWHM), and the detuning of the incident light from the atomic resonances is given by $\Delta_{ge}=\Omega-\omega_{ge}$. In the case of a conserved total atom population, one of the equations can be eliminated by the relation $\sum_g\rho^{(j)}_{gg}+\sum_e\rho^{(j)}_{ee}=1$. We have introduced a semiclassical approximation to factorize internal level two-body correlation functions. Due to this approximation, the ensemble average of many single realizations does not reproduce the nonclassical correlations in the system.

Instead of considering the full experimental configuration of all the $F=1,2$ and $F'=2$ electronic levels, we approximate the system in the numerical simulations by an effective three-level model where one of the ground levels refers to the initial state $|1\rangle\equiv|F,m_F\rangle=|2,2\rangle$, and all the final electronic ground levels are approximated by a single state $|2\rangle$. Resonant incident light then drives the transition $|1\rangle\leftrightarrow|e\rangle$ to an electronically excited state $|e\rangle$, and the atoms can spontaneously decay to both levels $|1\rangle$ and $|2\rangle$. For instance, when the transition strengths are equal for the two levels (and the atom can only decay for the two ground levels studied), the equations of motion then simplify to

$$\frac{d}{dt}\rho^{(j)}_{1e} = (i\Delta_{1e}-\Gamma)\rho^{(j)}_{1e} + i\frac{\xi}{\sqrt{2}\mathcal{D}}\rho^{(j)}_{11}\hat{\mathbf{e}}^*_1\cdot\mathbf{D}^+_F(\mathbf{X}_j) - i\frac{\xi}{\sqrt{2}\mathcal{D}}\rho^{(j)}_{ee}\hat{\mathbf{e}}^*_1\cdot\mathbf{D}^+_F(\mathbf{X}_j) + i\frac{\xi}{2}\sum_{l\neq j}\mathcal{G}^{(jl)}_{g'g}\rho^{(l)}_{ge}\rho^{(j)}_{1g'} - i\frac{\xi}{2}\sum_{l\neq j}\mathcal{G}^{(jl)}_{1g}\rho^{(l)}_{ge}\rho^{(j)}_{ee}, \quad (8a)$$

$$\frac{d}{dt}\rho^{(j)}_{2e} = (i\Delta_{2e}-\Gamma)\rho^{(j)}_{2e} + i\frac{\xi}{\sqrt{2}\mathcal{D}}\rho^{(j)}_{21}\hat{\mathbf{e}}^*_1\cdot\mathbf{D}^+_F(\mathbf{X}_j) + i\frac{\xi}{2}\sum_{l\neq j}\mathcal{G}^{(jl)}_{g'g}\rho^{(l)}_{ge}\rho^{(j)}_{2g'} - i\frac{\xi}{2}\sum_{l\neq j}\mathcal{G}^{(jl)}_{2g}\rho^{(l)}_{ge}\rho^{(j)}_{ee}, \quad (8b)$$

$$\frac{d}{dt}\rho^{(j)}_{12} = i\Delta_{12}\rho^{(j)}_{12} + \Gamma\rho^{(j)}_{ee} - i\frac{\xi}{\sqrt{2}\mathcal{D}}\rho^{(j)}_{e2}\hat{\mathbf{e}}^*_1\cdot\mathbf{D}^+_F(\mathbf{X}_j) - i\frac{\xi}{2}\sum_{l\neq j}\mathcal{G}^{(jl)}_{1g}\rho^{(l)}_{ge}\rho^{(j)}_{e2} + i\frac{\xi}{2}\sum_{l\neq j}[\mathcal{G}^{(jl)}_{2g}]^*\rho^{(l)}_{eg}\rho^{(j)}_{1e}, \quad (8c)$$

$$\frac{d}{dt}\rho^{(j)}_{11} = +\Gamma\rho^{(j)}_{ee} + \sqrt{2}\mathrm{Im}\big[\frac{\xi}{\mathcal{D}}\rho^{(j)}_{e1}\hat{\mathbf{e}}^*_1\cdot\mathbf{D}^+_F(\mathbf{X}_j)\big] + \mathrm{Im}\big[\xi\sum_{l\neq j}\mathcal{G}^{(jl)}_{1g}\rho^{(l)}_{ge}\rho^{(j)}_{e1}\big], \quad (8d)$$

$$\frac{d}{dt}\rho^{(j)}_{22} = +\Gamma\rho^{(j)}_{ee} + \mathrm{Im}\big[\xi\sum_{l\neq j}\mathcal{G}^{(jl)}_{2g}\rho^{(l)}_{ge}\rho^{(j)}_{e2}\big], \quad (8e)$$

$$\frac{d}{dt}\rho^{(j)}_{ee} = -2\Gamma\rho^{(j)}_{ee} - \sqrt{2}\mathrm{Im}\big[\frac{\xi}{\mathcal{D}}\rho^{(j)}_{e1}\hat{\mathbf{e}}^*_1\cdot\mathbf{D}^+_F(\mathbf{X}_j)\big] - \mathrm{Im}\big[\xi\sum_{l\neq j}\mathcal{G}^{(jl)}_{gg'}\rho^{(l)}_{g'e}\rho^{(j)}_{eg}\big], \quad (8f)$$

where the ground state symbols are again summed over.

The result is a set of coupled equations (8) for internal level one-body density matrix elements $\rho_{ab}^{(j)}$, for each atom $j = 1, \ldots, N$. In the absence of the radiative coupling terms $\mathcal{G}_{gg'}^{(jl)}$, with $g, g' = 1, 2$ the equations coincide with standard Bloch equations. The terms $\mathcal{G}_{gg'}^{(jl)}$ represent the strong resonant dipole-dipole interactions that depend on the relative positions between the atoms and lead to spatial correlations in the optical response. In the limit that the resonance frequencies of the different transitions differ considerably, the cross terms $\mathcal{G}_{gg'}^{(jl)}$, with $g \neq g'$ – that couple the different transitions $|1\rangle \leftrightarrow |e\rangle$ and $|2\rangle \leftrightarrow |e\rangle$ – become negligible. The standard two-level coupled dipole model approach [1, 4] is obtained from Eq. (8b) by setting all the terms involving $\rho_{ee}$ to zero and the indices $g = g' = 1$.

In the simulations, we then stochastically sample the set of discrete atomic coordinates $\{\mathbf{X}_1, \ldots, \mathbf{X}_N\}$ from the density distribution. For each realization we solve the semiclassical electrodynamics equations of motion (8) for all $\rho_{ab}^{(j)}$. Averaging over many such realizations allows the expectation values of desired observables to be computed. The simulations then incorporate all the recurrent scattering events between the atoms in a semi-classical approximation for random positions of the atoms.

During each stochastic realization the atoms are stationary. There are two timescales that would need to be taken into account. The first one, and the more important one, relates to light-mediated interactions and is determined by the time a single photon spends inside the sample, while undergoing multiple scattering events. This can be anything up to a few scattering events times the inverse resonance linewidth, and generally is less than 100ns. The thermal motion of the atoms on that timescale is negligible, and the atoms can be considered stationary.

The second time scale relates to the pulse duration and is significantly longer. It is possible that, due to the thermal motion of the atoms, in a single pulse different photons see different configurations of atomic positions. However, it turns out that the ensemble-averaging of the atomic positions between the different stochastic realizations of the pulse dynamics compensates for the atomic motion, and the effect is negligible in the optical response. We have explicitly tested this effect by interchanging the order of averaging: Instead of simulating in a single realization each pulse with one specific random configuration of atomic positions and then ensemble-averaging over many such pulses, we have also simulated the system by stochastically sampling many random atomic positions in regular intervals during each pulse, before ensemble-averaging over many runs. In other words, we divided the pulse over a number of time intervals after each of which we randomised the atomic positions before continuing the pulse dynamics. We found that interchanging the order of averaging had a negligible effect on the population decay (much less than 1%).

TABLE I. Simulated atom numbers for each trap volume and the corresponding peak atom densities.

| $V/V_e$ | $N$ | $10^{-3}\rho/k^3$ |
|---|---|---|
| 1 | 12, 18, 25, 35 | 18, 27, 38, 53 |
| 0.35 | 8, 12, 15 | 34, 51, 63 |
| 0.072 | 3, 6, 9 | 62, 120, 190 |
| 0.023 | 3, 4, 5, 7 | 200, 270, 330, 470 |

The quantitative comparison between the simulated and experimental results is made via the saturation parameter, defined as $s = \Omega_R^2/2\Gamma^2$, with $\Omega_R$ the Rabi frequency and $\Gamma = 2\pi \times 3.03$ MHz HWHM. In Eqs. (8) above, the Rabi frequency is given by $\Omega_R = (\xi\sqrt{2}/\mathcal{D}) \left|\hat{\mathbf{e}}_1^* \cdot \mathbf{D}_F^+(\mathbf{X}_j)\right|$. The experimental value of $s$ is obtained as $s = (1/12) I/I_s$, with $I_s = 1.67$ mW/cm$^2$. The factor $1/12$ is the product of three factors: $1/2$ from projection onto $\sigma^+$ polarization component; $1/2$ from the (squared) reduced dipole moment of the $F = 2 \rightarrow F' = 2$ hyperfine component; $1/3$ from the squared Clebsch-Gordan coefficient of the $|2, 2\rangle \rightarrow |2', 1'\rangle$ transition.

Finally, in order to generate the results shown in the figures of the main section, we calculate in the simulations the remaining population in the initial state $\rho_{11}$ as a function of time. This yields exponential decay rates (calculated from the initial population and from the $t = 500/\Gamma$ results), or the pumping rates, each of which is represented by a single data point in Fig. 4(a) of the main text. The different data sets in Fig. 4 are obtained for different cloud volumes, resulting in the variation of both the atom density and optical thickness. Table I shows the simulated atom numbers for atom clouds whose volumes are smaller by the factor $V/V_e$ than the experimental value (the aspect ratios are the same in all cases).

## NUMBER OF ATOMS CALCULATION

In this experiment we use absorption imaging in order to measure the optical thickness of the atomic clouds. The optical thickness is then converted to number of atoms per pixel. This conversion depends on the camera pixel size, the magnification, and the absorption cross section $\sigma$. Our camera's pixel size and magnification are known (13 $\mu$m and 13, respectively), but $\sigma$ should be simulated. For an imaging laser with $\sigma^+$ polarization driving the $|2, 2\rangle \rightarrow |3, 3\rangle$ transition $\sigma_0 = 3\lambda^2/2\pi$. In our system, however, the initial state is a distribution over the $m_F$ states of the $F = 2$ ground state, and the imaging polarization is $\pi$. In addition, the atomic distribution in the ground state changes during the imaging pulse. In

order to find the effective cross section $\sigma_{\rm eff}$ (time averaged over the imaging pulse) we solve the optical Bloch equations (OBE) for the 12 relevant states (5 Zeeman sublevels of the $F = 2$ ground state, and 7 for the $F' = 3$ excited state) using our experimental parameters ($s \ll 1$ and $B = 5.4\,$G) with different initial conditions (initial distribution). We find that

$$\sigma_{\rm eff} = (0.15 \pm 0.02)\sigma_0. \qquad (9)$$

The error in $\sigma_{\rm eff}$ is due to the different initial distributions, and it is the main contribution to the error bars in number of atoms in the figures (the other source of error is shot-to-shot fluctuations). We would like to note that $\sigma_{\rm eff}$ includes a factor 0.5 to compensate the retro-reflecting imaging scheme we use.

In order to improve our image quality and lower the noise in the image and the number of atoms we use two more algorithms: fringe removal and deconvolution. The fringe removal algorithm [5] takes an array of images of the imaging laser with no atomic cloud and generates a new image, which is a linear combination of these images, that minimizes the fringe visibility in the optical density image. This minimization is done in an area with no atoms, and the linear combination has different weights for each measurement. This algorithm deals with the main noise contribution that comes from fringes due to spurious reflections, which does not cancel well in the optical density image. It assumes that if these fringes will be canceled in the area near the atoms, this cancelation will be valid also in the area with atoms.

The second algorithm, the deconvolution, is performed because signal from one microtrap 'leaks' to neighboring sites. This leakage is a convolution of the 'real' number of atoms with a point-spread-function (PSF). Using a second order correlation matrix $g^{(2)}$ we confirm that the signal in each trap depends on its neighboring sites. We also find, using a fitting algorithm, a PSF that creates the same dependence of a site on it neighbors (the correlation matrix). The last step is to deconvolute our images with the fitted PSF. We would like to note that here we do not use the single pixels of the CCD. We rather sum a square around each microtrap [the square in Fig. 1] and use it as a 'pixel' for the deconvolution algorithm. The deconvoluted number of atoms is presented in figures 2 and 3 in the main text of the paper.

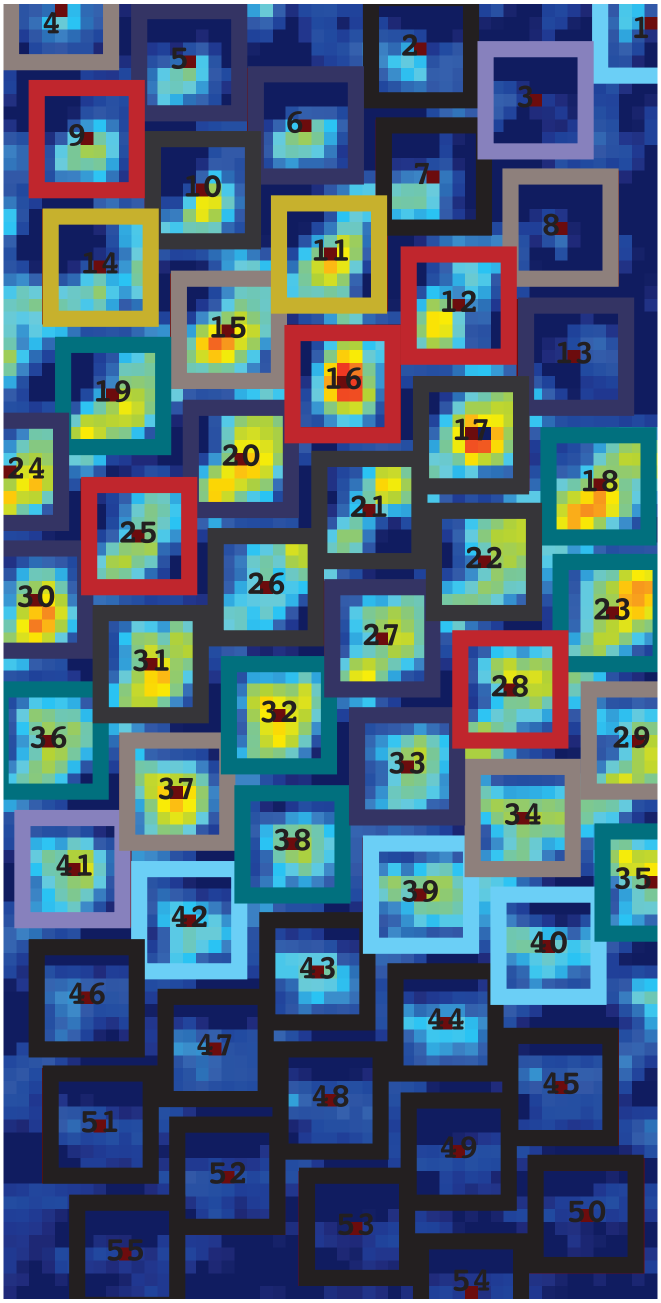

FIG. 1. The analysis area. Each microtrap center is marked with a red dot and a site index. The squares around the microtraps represent the area where we count the atoms, and the colors indicate the groups (see Table II). Traps that appear to be cut still use a full-size square to count the number of atoms by counting the relevant area outside the image shown here.

## MICROTRAPS GROUPS

The analysis in this work was not done on a single cloud level, but rather on groups of clouds. This was done in order to reduce noise. The grouping was done based on the initial number of atoms in each site, which is averaged over 26 images. Figure 1 shows the area where we perform our analysis, and the individual microtraps. The pumping time is zero in the figure, and it shows the initial microtraps densities. The color of the square indicates the group, see Table II for site indexes for each group. The sites marked with black squares are ignored because of low atom number.

TABLE II. Grouping of microtraps based on initial number of atoms.

| | site index | $N_0$ |
|---|---|---|
| group 1 | 1, 39, 40, 42 | $33 \pm 5$ |
| group 2 | 3, 41 | $58 \pm 8$ |
| group 3 | 4, 8, 15, 29, 34, 37 | $84 \pm 11$ |
| group 4 | 18, 19, 23, 32, 35, 36, 38 | $103 \pm 14$ |
| group 5 | 5, 6, 20, 24, 27, 30 | $131 \pm 18$ |
| group 6 | 10, 13, 33 | $157 \pm 21$ |
| group 7 | 17, 21, 22, 26, 31 | $181 \pm 24$ |
| group 8 | 9, 12, 16, 25, 28 | $204 \pm 27$ |
| group 9 | 11, 14 | $232 \pm 31$ |

[1] Juha Javanainen, Janne Ruostekoski, Bjarne Vestergaard, and Matthew R. Francis, "One-dimensional modelling of light propagation in dense and degenerate samples," Phys. Rev. A **59**, 649–666 (1999).

[2] Mark D. Lee, Stewart D. Jenkins, and Janne Ruostekoski, "Stochastic methods for light propagation and recurrent scattering in saturated and nonsaturated atomic ensembles," Phys. Rev. A **93**, 063803 (2016).

[3] John David Jackson, *Classical Electrodynamics*, 3rd ed. (Wiley, New York, 1999).

[4] Stewart D. Jenkins and Janne Ruostekoski, "Controlled manipulation of light by cooperative response of atoms in an optical lattice," Phys. Rev. A **86**, 031602 (2012).

[5] C. F. Ockeloen, A. F. Tauschinsky, R. J. C. Spreeuw, and S. Whitlock, "Detection of small atom numbers through image processing," Phys. Rev. A **82**, 061606 (2010).
